# Supplementary material for: Fairness in Multi-Agent Planning
Source: arXiv:2212.00506 source file (2023-05-22)
Supplement: Supplementary file 1 [file appendix_main.tex]

%File: formatting-instruction.tex
\documentclass[letterpaper]{article}
\usepackage[submission]{aaai23}  % DO NOT CHANGE THIS
\usepackage{times}  % DO NOT CHANGE THIS
\usepackage{helvet}  % DO NOT CHANGE THIS
\usepackage{courier}  % DO NOT CHANGE THIS
\usepackage[hyphens]{url}  % DO NOT CHANGE THIS
\usepackage{graphicx} % DO NOT CHANGE THIS
\urlstyle{rm} % DO NOT CHANGE THIS
  % DO NOT CHANGE THIS
\usepackage{natbib}  % DO NOT CHANGE THIS AND DO NOT ADD ANY OPTIONS TO IT
\usepackage{caption} % DO NOT CHANGE THIS AND DO NOT ADD ANY OPTIONS TO IT
\frenchspacing  % DO NOT CHANGE THIS
\setlength{\pdfpagewidth}{8.5in} % DO NOT CHANGE THIS
\setlength{\pdfpageheight}{11in} % DO NOT CHANGE THIS

\usepackage{algorithm}
\usepackage{algorithmic}
\usepackage{breqn}

%
% These are are recommended to typeset listings but not required. See the subsubsection on listing. Remove this block if you don't have listings in your paper.
\usepackage{newfloat}
\usepackage{listings}
\DeclareCaptionStyle{ruled}{labelfont=normalfont,labelsep=colon,strut=off} % DO NOT CHANGE THIS
\lstset{%
	basicstyle={\footnotesize\ttfamily},% footnotesize acceptable for monospace
	%numbers=left,numberstyle=\footnotesize,xleftmargin=2em,% show line numbers, remove this entire line if you don't want the numbers.
	aboveskip=0pt,belowskip=0pt,%
	showstringspaces=false,tabsize=2,breaklines=true}
\floatstyle{ruled}
\newfloat{listing}{tb}{lst}{}
\floatname{listing}{Listing}
\usepackage{graphicx}
\usepackage{mathtools}
\usepackage{xcolor}
\usepackage{amsmath}
\usepackage{amsthm}
\usepackage{amssymb}
\usepackage{adjustbox}
\usepackage{pifont}% http://ctan.org/pkg/pifont
\usepackage{url}
\usepackage{makecell}
\usepackage{multirow}\usepackage{multicol}

%%%%%%%% COSAS LISTINGS Y PDDL %%%%
\lstdefinelanguage{pddl}
{
    keywords={
        define,
    },
    keywordstyle=[2]{\color{red}},
    morekeywords={[2]
        domain,
        problem,
        requirements,
        predicates,
        types,
        action,
        init,
        goal,
        typing,
        costs,
        functions,
    },
    keywordstyle=[3]{\color{blue}},
    morekeywords={[3]
        parameters,
        vars,
        precondition,
        effect,
        duration,
    },
    keywordstyle={[4]\color{olive}},
    morekeywords={[4]
        forall,
        or,
        and,
        not,
        when,
        =,
        exists,
        at start,
        at end,
        over all,
        imply,
        oneof,
        increase,
    },
    comment=[l]{\;},
    sensitive=true
}[keywords, comments]

\lstdefinelanguage[mapl]{pddl}[]{pddl}
{
    morekeywords={[2]
      sensor,
    },
    morekeywords={[3]
      sense,
      replan
    },
    morekeywords={[4]
      KIF,
    },
}

% \lstset{
% 	emph={\:predicates,\:metric, \:derived,\:action,\:goal,\:init,\:objects,\:functions,\:types}, emphstyle=\color{BrickRed},
% 	emph={[2]\:parameters,\:precondition,\:effectl,oneof},emphstyle={[2]\color{OliveGreen}},
% 	emph={[3]exists,not,forall,minimize,when,increase,decrease,and,or},emphstyle={[3]\color{mymauve}}
% }
% \lstset{basicstyle=\small\ttfamily} 

% 
% 
% \lstset{
%   basicstyle=\ttfamily\small,
%   mathescape=true,
%   keywordstyle={\color{BrickRed}},
%   morekeywords={action},
%   keywordstyle=[2]{\color{OliveGreen}},
%   morekeywords=[2]{precondition,effect},
%   keywordstyle=[3]{\color{MidnightBlue}},
%   morekeywords=[3]{and,when,or,not,oneof}
% }

\lstset{language=pddl}
\lstset{basicstyle=\small\ttfamily} 
\lstset{basicstyle=\scriptsize\ttfamily}

\usepackage{color}

 \begin{document}
\onecolumn
\include{appendix}
\end{document}
